# Supplementary material for: ELSA: Efficient Long-Term Secure Storage of Large Datasets
Source: arXiv:1810.11888 source file (2018-10-28)
Supplement: Supplementary file 1 [file appendix.tex]

%!TEX root = ../main.tex

\section{Proofs}

\printallsaved{proof}

%\printproofs

\section{Algorithms}

\printallsaved{algorithm}
